# Supplementary material for: Provable Dynamic Fusion for Low-Quality Multimodal Data
Source: arXiv:2306.02050 source file (2023-06-06)
Supplement: Supplementary file 2 [file tab-classification.tex]

\begin{table*}[!t]
\small
\vspace{0.0cm}
% \vskip 0.35in
\begin{center}
% \begin{spacing}{1.05}   
\caption{Supplement to Table \ref{tab:classification} with more cases. Classification accuracy performance comparison when 50\% of the modalities is corrupted with Salt-peper noise with varying signal noise rate $\epsilon$).}
\label{tab:classification-pepper}
\center
{

\begin{tabular}{c|c|c|c|cccccc}
\toprule
\multicolumn{1}{c}{\text{Dataset}}  &\multicolumn{1}{c}{\text{Modality}}  & \multicolumn{1}{c}{\text{Method}}  & \multicolumn{1}{c}{\text{QMI}}  &
\text{$\mathbf{\epsilon=0.0}$}& \text{\begin{tabular}[c]{@{}c@{}}$\mathbf{\epsilon=0.1}$\\ \end{tabular}}& \text{\begin{tabular}[c]{@{}c@{}}$\mathbf{\epsilon=0.2}$\\ \end{tabular}}& \text{\begin{tabular}[c]{@{}c@{}}$\mathbf{\epsilon=0.3}$\\ \end{tabular}}& \text{\begin{tabular}[c]{@{}c@{}}$\mathbf{\epsilon=0.5}$\\ \end{tabular}}
\\ \toprule
 \multirow{12}{*} {\text{NYUD2}} & {\text{RGB}}  
    &   \multirow{2}{*}{\text{Uni-modal}}      & \xmark                                         &${63.42\pm0.69}$  &${53.30\pm0.81}$
       &${45.78\pm1.17}$   
       &${39.48\pm2.01}$
       &${38.59\pm1.94}$ \\
                                                                     &        {\text{Depth}}      &  & \xmark            
                                                         &${62.14\pm1.40}$   
                                                         &${52.51\pm1.72}$   
                                                         &${45.14\pm2.92}$   
                                                         &${37.37\pm3.25}$ 
                                                         &${35.72\pm2.23}$                                    \\ \cline{2-9} & \multirow{11}{*} {\text{RGB-D}}
      &  \multirow{3}{*}{\text{LF}}       & \xmark                                                    &$69.11\pm0.72$ &$66.51\pm0.53$ &$63.67\pm0.53$   &$60.80\pm1.78$   &$55.75\pm2.42$    \\
                                                                                  
                                                 &           &                           & \cmark                                                                                            &${70.92\pm1.56}$   &${69.69\pm1.71}$ &${68.23\pm1.73}$   &${66.09\pm1.73}$  &${62.14\pm2.27}$   \\& & & Improve & \textcolor{mycolor2}{{$~~~~~~~~\bigtriangleup 1.81 $}} & \textcolor{mycolor2}{{$~~~~~~\bigtriangleup 3.18 $}}&\textcolor{mycolor2}{{$~~~~~~\bigtriangleup 4.56 $}}& \textcolor{mycolor2}{{$~~~~~~\bigtriangleup 5.29 $}}  & \textcolor{mycolor2}{{$~~~~~~\bigtriangleup 2.63 $}}                               \\\cline{3-9}
&     &  \multirow{3}{*}{\text{Concat}}      & \xmark                                                      &${70.12\pm0.39}$  &${68.10\pm0.94}$ &${65.81\pm1.19}$  &${63.30\pm1.27}$  &${58.29\pm2.20}$                                         \\
                                                                   &              &             & \cmark                                                       &${70.00\pm1.23}$  &${68.35\pm1.45}$ &${67.16\pm1.18}$   &${65.08\pm1.18}$         &${60.92\pm2.22}$                        \\& & & Improve & {-} & \textcolor{mycolor2}{{$~~~~~~\bigtriangleup 0.25 $}}&\textcolor{mycolor2}{{$~~~~~~\bigtriangleup 1.35 $}}& \textcolor{mycolor2}{{$~~~~~~\bigtriangleup 1.78 $}}  &  \textcolor{mycolor2}{{$~~~~~~\bigtriangleup 2.63 $}}      \\  \cline{3-9}
    & &  \multirow{3}{*}{\text{Align}}      & \xmark                                                      &${71.36\pm1.41}$  &${69.24\pm1.66}$ &${67.15\pm1.60}$  &${64.53\pm2.23}$  &${59.45\pm2.29}$                                         \\
                                                                            &     &             & \cmark                                                       &${71.13\pm0.38}$  &${69.88\pm0.57}$ &${68.53\pm1.30}$  &${66.67\pm1.66}$  &${63.00\pm1.33}$                        \\& & & Improve & {-} & \textcolor{mycolor2}{{$~~~~~~\bigtriangleup 0.64 $}}&\textcolor{mycolor2}{{$~~~~~~\bigtriangleup 1.38 $}}& \textcolor{mycolor2}{{$~~~~~~\bigtriangleup 2.14 $}}  &  \textcolor{mycolor2}{{$~~~~~~\bigtriangleup 3.55 $}}                                                                              \\ \cline{3-9}
&     &  \multirow{3}{*}{\text{MMTM}}      & \xmark                                                      &${71.04\pm0.16}$ &${68.38\pm0.68}$ &${65.87\pm1.07}$  &${63.61\pm1.37}$  &${59.54\pm1.24}$                                         \\
                                                                   &              &             & \cmark                                                       &${71.25\pm0.31}$ &${70.06\pm0.56}$ &${68.56\pm0.27}$   &${67.06\pm0.63}$         &${64.16\pm0.65}$                        \\& & & Improve & {-} & \textcolor{mycolor1}{{$~~~~~~~~\bigtriangleup 1.68 $}} &\textcolor{mycolor2}{{$~~~~~~\bigtriangleup 2.79 $}}& \textcolor{mycolor2}{{$~~~~~~\bigtriangleup 3.45 $}}  &  \textcolor{mycolor2}{{$~~~~~~\bigtriangleup 4.62 $}}\\ \midrule  \multirow{12}{*} {\text{SUN}} & {\text{RGB}}  
    &   \multirow{2}{*}{\text{Uni-modal}}      & \xmark                                         &${57.49\pm0.58}$  
    &${49.13\pm0.44}$
       &${43.51\pm0.77}$   
       &${39.61\pm0.98}$
       &${37.29\pm0.87}$ \\
                                                                     &        {\text{Depth}}      &  & \xmark            
                                                         &${53.88\pm0.57}$
                                                         &${38.52\pm1.84}$
                                                         &${33.31\pm1.63}$   
                                                         &${29.33\pm0.33}$ 
                                                         &${28.46\pm0.12}$                                    \\ \cline{2-9} & \multirow{11}{*} {\text{RGB-D}}
      &  \multirow{3}{*}{\text{LF}}       & \xmark                                                   &$62.00\pm0.15$  &$52.67\pm1.45$ &$51.72\pm1.32$   &$51.05\pm0.96$   &$51.05\pm0.82$    \\
                                                                                  
                                                 &           &                           & \cmark                                                                                            &${62.22\pm0.34}$   &${60.65\pm0.15}$ &${58.87\pm0.43}$   &${57.02\pm0.69}$  &${53.38\pm1.18}$   \\& & & Improve & \textcolor{mycolor2}{{$~~~~~~~~\bigtriangleup 0.22 $}} & \textcolor{mycolor2}{{$~~~~~~\bigtriangleup 7.98 $}}& \textcolor{mycolor2}{{$~~~~~~\bigtriangleup 7.15 $}}  & \textcolor{mycolor2}{{$~~~~~~\bigtriangleup 5.97 $}}     & \textcolor{mycolor2}{{$~~~~~~\bigtriangleup 2.33 $}}                           \\\cline{3-9}
&     &  \multirow{3}{*}{\text{Concat}}      & \xmark                                                      &${62.48\pm0.50}$  &${60.24\pm0.29}$ &${58.01\pm0.53}$  &${55.92\pm0.92}$  &${51.00\pm1.42}$                                         \\
                                                                   &              &             & \cmark                                                       &${61.90\pm0.40}$  &${60.67\pm0.34}$ &${59.26\pm0.55}$  &${57.78\pm0.69}$  &${54.42\pm0.94}$                        \\& & & Improve & \textcolor{mycolor2}{{$~~~~~~~~\bigtriangledown 0.58 $}} & \textcolor{mycolor2}{{$~~~~~~\bigtriangleup 0.43 $}}& \textcolor{mycolor2}{{$~~~~~~\bigtriangleup 1.25 $}}  &  \textcolor{mycolor2}{{$~~~~~~\bigtriangleup 1.86 $}}  &  \textcolor{mycolor2}{{$~~~~~~\bigtriangleup 3.42 $}}      \\  \cline{3-9}
    & &  \multirow{3}{*}{\text{Align}}      & \xmark                                                      &${61.22\pm0.66}$  &${59.18\pm0.76}$ &${57.37\pm1.06}$  &${55.38\pm0.98}$  &${51.05\pm1.24}$                                         \\
                                                                            &     &             & \cmark                                                       &${62.39\pm0.54}$
                                                                            &${60.93\pm0.53}$ &${59.46\pm0.78}$   &${57.84\pm1.15}$         &${54.44\pm1.41}$                        \\& & & Improve & \textcolor{mycolor2}{{$~~~~~~~~\bigtriangleup 1.17 $}} & \textcolor{mycolor2}{{$~~~~~~\bigtriangleup 1.75 $}}& \textcolor{mycolor2}{{$~~~~~~\bigtriangleup 2.09 $}}  &  \textcolor{mycolor2}{{$~~~~~~\bigtriangleup3.46 $}}    &  \textcolor{mycolor2}{{$~~~~~~\bigtriangleup3.39 $}}                                                                          \\ \cline{3-9}
&     &  \multirow{3}{*}{\text{MMTM}}      & \xmark                                                      &${61.72\pm0.67}$  &${59.68\pm0.62}$ &${57.37\pm0.43}$  &${55.17\pm0.35}$  &${50.83\pm0.81}$                                         \\
                                                                   &              &             & \cmark                                                       &${62.70\pm0.30}$
                                                                   &${61.55\pm0.45}$
                                                                   &${60.56\pm0.55}$   &${59.09\pm0.33}$         &${55.83\pm0.43}$                       \\& & & Improve & \textcolor{mycolor2}{{$~~~~~~~~\bigtriangleup 0.98 $}} & \textcolor{mycolor2}{{$~~~~~~\bigtriangleup 1.97 $}}& \textcolor{mycolor2}{{$~~~~~~\bigtriangleup 3.29 $}}  &  \textcolor{mycolor2}{{$~~~~~~\bigtriangleup3.82 $}}    &  \textcolor{mycolor2}{{$~~~~~~\bigtriangleup5.00 $}}\\

\bottomrule
\end{tabular}}
% \end{spacing}
\end{center}
\vspace{0mm}
\end{table*}
