# Supplementary material for: Provable Dynamic Fusion for Low-Quality Multimodal Data
Source: arXiv:2306.02050 source file (2023-06-06)
Supplement: Supplementary file 3 [file tab-sun-seg.tex]

\begin{table*}[!htbp]\small
\vspace{0.0cm}
% \vskip 0.35in
\begin{center}
% \begin{spacing}{1.05}   
\caption{Mean intersection over union (MIoU) comparison on \textbf{SUN-RGBD} dataset when 50\% of the modalities is corrupted with Gaussian noise (i.e., zero mean with varying variance $\epsilon$).}
\label{tab:sun-segmentation-noise}
\center

{

\begin{tabular}{c|c|c|c|cccccc}
\toprule
\multicolumn{1}{c}{\text{Dataset}}  &\multicolumn{1}{c}{\text{Modality}}  & \multicolumn{1}{c}{\text{Method}}  & \multicolumn{1}{c}{\text{QMI}}  &
\text{$\mathbf{\epsilon=0.0}$}& \text{\begin{tabular}[c]
{@{}c@{}}$\mathbf{\epsilon=5.0}$\\ \end{tabular}}& \text{\begin{tabular}[c]{@{}c@{}}$\mathbf{\epsilon=10.0}$\\ \end{tabular}}& \text{\begin{tabular}[c]{@{}c@{}}$\mathbf{\epsilon=20.0}$\\ \end{tabular}}& \text{\begin{tabular}[c]{@{}c@{}}$\mathbf{\epsilon=30.0}$\\ \end{tabular}}
\\ \toprule \multirow{10}{*}{\shortstack{\text{SUN-}\\\text{RGBD}}}&
{\text{RGB}}  
    &   \multirow{2}{*}{\text{Uni-modal}}      & \xmark                                         &${42.76}$  
       &${41.77}$   
       &${38.36}$
       &${32.20}$
       &${28.55}$ \\&
                                                                             {\text{Depth}}      &  & \xmark            
                                                         &${38.42}$   
                                                         &${34.39}$   
                                                         &${30.18}$ 
                                                         &${26.88}$
                                                         &${24.54}$                                    \\ \cline{2-9} & \multirow{8}{*} {\text{RGB-D}}
      &  \multirow{3}{*}{\text{Late fusion}}       & \xmark                                                    &$45.17$  &$43.00$   &$38.13$   &$30.49$ &$28.56$   \\
                                                                                  
                                                            &  &                         & \cmark                                                                                            &${45.01}$   &${43.34}$   &${41.25}$  &${37.20}$
                                                            &${34.89}$ 
                                                            \\& & & Improve & {-} & \textcolor{mycolor2}{{$\bigtriangleup 0.34 $}}&
                                                            \textcolor{mycolor2}{{$\bigtriangleup 3.12 $}}  &
                                                            \textcolor{mycolor2}{{$\bigtriangleup 6.71 $}}  & \textcolor{mycolor2}{{$\bigtriangleup 6.33 $}}                                     \\ \cline{3-9}
  &   &  \multirow{3}{*}{\text{SE-add}}      & \xmark                                                      &${46.95}$  &${44.93}$  &${40.64}$  &${32.93}$   &${27.72}$                                         \\&
                                                                                 &             & \cmark                                                       &${47.08}$  &${46.23}$   &${44.08}$         &${40.73}$   &${38.58}$                      \\& & & Improve & \textcolor{mycolor1}{{$\bigtriangledown 0.13 $}} & \textcolor{mycolor2}{{$\bigtriangleup 1.30 $}}& \textcolor{mycolor2}{{$\bigtriangleup 3.44 $}}  &  \textcolor{mycolor2}{{$\bigtriangleup 7.80 $}}  &  \textcolor{mycolor2}{{$\bigtriangleup 10.86 $}}                                                                              \\\cline{3-9}
   &  &  \multirow{3}{*}{\text{ESA-Net}}      & \xmark                                                      &${47.45}$  &${45.55}$  &${41.51}$  &${33.48}$   &${28.52}$                                \\&
                                                                                 &             & \cmark                                                       &${46.48}$  &${45.91}$   &${43.68}$         &${37.46}$ &${31.19}$           \\& & & Improve & \textcolor{mycolor1}{{$\bigtriangledown 0.97 $}} & \textcolor{mycolor2}{{$\bigtriangleup 0.36 $}}& \textcolor{mycolor2}{{$\bigtriangleup 2.17 $}}  &  \textcolor{mycolor2}{{$\bigtriangleup 3.98 $}} &
                                                                                 \textcolor{mycolor2}{{$\bigtriangleup 2.67 $}}\\  \bottomrule
\end{tabular}}
% \end{spacing}
\end{center}
\vspace{0.0mm}
\end{table*}
