# Supplementary material for: Provable Dynamic Fusion for Low-Quality Multimodal Data
Source: arXiv:2306.02050 source file (2023-06-06)
Supplement: Supplementary file 4 [file comparison-nyud2.tex]

\begin{table*}[!htbp]\small
\vspace{0.0cm}
% \vskip 0.35in
\begin{center}
% \begin{spacing}{1.05}   
\caption{Comparison with other uncertainty-based multimodal fusion methods.}
\label{tab:comparison-nyud2}
\center

{

\begin{tabular}{c|c|c|ccccc}
\toprule
\multicolumn{1}{c}{\text{Dataset}}  &\multicolumn{1}{c}{\text{Modality}}  & \multicolumn{1}{c}{\text{Approach}}    &
\text{$\mathbf{\epsilon=0.0}$}& \text{\begin{tabular}[c]
{@{}c@{}}$\mathbf{\epsilon=0.1}$\\ \end{tabular}}& \text{\begin{tabular}[c]{@{}c@{}}$\mathbf{\epsilon=0.2}$\\ \end{tabular}}& \text{\begin{tabular}[c]{@{}c@{}}$\mathbf{\epsilon=0.3}$\\ \end{tabular}}& \text{\begin{tabular}[c]{@{}c@{}}$\mathbf{\epsilon=0.5}$\\ \end{tabular}}
\\ \toprule \multirow{5}{*}{\text{NYUD2}}&
{\text{RGB}}  
    &   \multirow{2}{*}{\text{Uni-modal}}                                               &${63.42\pm0.69}$  &${60.73\pm0.98}$  &${57.86\pm1.21}$  &${55.54\pm1.12}$   &${50.49\pm1.17}$ \\&
                                                                             {\text{Depth}}      &              
                                                         &${62.14\pm1.40}$  &${58.99\pm1.52}$  &${56.64\pm1.54}$  &${53.98\pm1.81}$   &${48.56\pm1.18}$                                    \\ \cline{2-8} & \multirow{3}{*} {\text{RGB-D}}
      &  \multirow{1}{*}{\text{Late fusion}}                                                         &${69.11\pm0.72}$  &${66.51\pm0.53}$  &${63.67\pm0.78}$  &${60.80\pm1.78}$   &${55.75\pm2.42}$                                        \\ 
  &   &  \multirow{1}{*}{\text{TMC}}                                                          &${70.64\pm0.77}$  &${68.81\pm0.72}$  &${66.97\pm0.80}$  &${64.77\pm0.80}$   &${59.33\pm0.90}$                                                                                                                      \\
   &  &  \multirow{1}{*}{\text{QMF(LF)}}                                                          &  \textcolor{blue}{${70.92\pm1.56}$} &\textcolor{blue}{${69.69\pm1.71}$}  &\textcolor{blue}{${68.23\pm1.73}$}  &\textcolor{blue}{${66.09\pm1.78}$}   &\textcolor{blue}{${62.14\pm2.27}$}                                \\  \bottomrule
\end{tabular}}
% \end{spacing}
\end{center}
\vspace{0.0mm}
\end{table*}
