# Supplementary material for: Provable Dynamic Fusion for Low-Quality Multimodal Data
Source: arXiv:2306.02050 source file (2023-06-06)
Supplement: Supplementary file 5 [file comparison-sun.tex]

\begin{table*}[!htbp]\small
\vspace{0.0cm}
% \vskip 0.35in
\begin{center}
% \begin{spacing}{1.05}   
\caption{Comparison with other uncertainty-based multimodal fusion methods.}
\label{tab:comparison-sun}
\center

{

\begin{tabular}{c|c|c|ccccc}
\toprule
\multicolumn{1}{c}{\text{Dataset}}  &\multicolumn{1}{c}{\text{Modality}}  & \multicolumn{1}{c}{\text{Approach}}    &
\text{$\mathbf{\epsilon=0.0}$}& \text{\begin{tabular}[c]
{@{}c@{}}$\mathbf{\epsilon=0.1}$\\ \end{tabular}}& \text{\begin{tabular}[c]{@{}c@{}}$\mathbf{\epsilon=0.2}$\\ \end{tabular}}& \text{\begin{tabular}[c]{@{}c@{}}$\mathbf{\epsilon=0.3}$\\ \end{tabular}}& \text{\begin{tabular}[c]{@{}c@{}}$\mathbf{\epsilon=0.5}$\\ \end{tabular}}
\\ \toprule \multirow{5}{*}{\text{SUN-RGBD}}&
{\text{RGB}}  
    &   \multirow{2}{*}{\text{Uni-modal}}                                               &$57.49\pm0.58$  &$55.23\pm0.76$   &$53.07\pm0.87$   &$50.80\pm0.80$ &$46.60\pm0.77$ \\&
                                                                             {\text{Depth}}      &              
                                                         &$53.88\pm0.57$  &$51.40\pm0.53$   &$48.94\pm0.89$   &$46.43\pm1.02$ &$41.29\pm1.10$                                    \\ \cline{2-8} & \multirow{3}{*} {\text{RGB-D}}
      &  \multirow{1}{*}{\text{Late fusion}}                                                         &$62.00\pm0.15$  &$52.67\pm1.45$   &$51.67\pm1.32$   &$51.05\pm0.96$ &$51.05\pm0.82$                                        \\ 
  &   &  \multirow{1}{*}{\text{TMC}}                                                          &$62.00\pm0.15$  &$52.67\pm1.45$   &$51.67\pm1.32$   &$51.05\pm0.96$ &$51.05\pm0.82$                                                                                                                      \\
   &  &  \multirow{1}{*}{\text{QMF(LF)}}                                                            &\textcolor{blue}{$62.22\pm0.34$}  &\textcolor{blue}{$60.65\pm0.15$}   &\textcolor{blue}{$58.87\pm0.43$}   &\textcolor{blue}{$57.02\pm0.69$} &\textcolor{blue}{$53.38\pm1.18$}                                \\  \bottomrule
\end{tabular}}
% \end{spacing}
\end{center}
\vspace{0.0mm}
\end{table*}
