# Supplementary material for: Provable Dynamic Fusion for Low-Quality Multimodal Data
Source: arXiv:2306.02050 source file (2023-06-06)
Supplement: Supplementary file 6 [file tab-ablation-LF.tex]

\begin{table}[!htbp]
\vspace{-0.2cm}
% \vskip 0.35in
\begin{center}
% \begin{spacing}{1.05}   
\caption{Ablation study for different combinations of objective components, where it is realized by using late fusion as the backbone.}
\label{tab:nyud2-LF-ablation}
\center
{
\setlength{\tabcolsep}{1.9mm}
\begin{tabular}{ccc|ccccc}
\toprule
\multicolumn{1}{c}{\text{Sampling}}  & \multicolumn{1}{c}{\text{QAW}}  & \multicolumn{1}{c}{\text{$L_{reg}$}}  &
\text{$\mathbf{\epsilon=0.0}$}& \text{\begin{tabular}[c]{@{}c@{}}$\mathbf{\epsilon=10.0}$\\ \end{tabular}}& \text{\begin{tabular}[c]{@{}c@{}}$\mathbf{\epsilon=20.0}$\\ \end{tabular}}& \text{\begin{tabular}[c]{@{}c@{}}$\mathbf{\epsilon=30.0}$\\ \end{tabular}}
\\ \midrule
  
 \xmark   &\xmark         &\xmark                                          &${70.95}$  
       &${49.69}$   
       &${45.87}$
       &${43.88}$ \\
                                                                             \cmark      &\xmark  &\xmark             
                                                         &${70.34}$  
       &${57.34}$   
       &${54.13}$
       &${51.99}$                                    \\  \xmark      &\cmark  &\xmark             
                                                         &${69.11}$   
                                                         &${50.61}$   
                                                         &${45.26}$ 
                                                         &${45.41}$          \\  \xmark      &\xmark  &\cmark             
                                                         &${70.18}$   
                                                         &${51.22}$   
                                                         &${45.87}$ 
                                                         &${45.57}$             \\  \cmark      &\cmark  &\xmark             
                                                         &${70.64}$   
                                                         &${58.41}$   
                                                         &${55.05}$ 
                                                         &${52.75}$      \\  \cmark      &\xmark  &\cmark             
                                                         &${71.71}$   
                                                         &$\pmb{59.02}$   
                                                         &${55.05}$ 
                                                         &${54.43}$     \\  \xmark      &\cmark  &\cmark             
                                                         &${70.33}$   
                                                         &${50.77}$   
                                                         &${47.09}$ 
                                                         &${45.57}$   \\\midrule \cmark      &\cmark  & \cmark            
                                                         &$\pmb{72.17}$   
                                                         &${{58.86}}$  
                                                         &${\pmb{55.35}}$
                                                         &${\pmb{54.74}}$                                   \\ \bottomrule
\end{tabular}}
% \end{spacing}
\end{center}
\vspace{-0.4cm}
\end{table}
