# Supplementary material for: Provable Dynamic Fusion for Low-Quality Multimodal Data
Source: arXiv:2306.02050 source file (2023-06-06)
Supplement: Supplementary file 7 [file tab-ablation-MMTM.tex]

\begin{table}[!htbp]
\vspace{-0.2cm}
% \vskip 0.35in
\begin{center}
% \begin{spacing}{1.05}   
\caption{Ablation study for different combinations of objective components, where it is realized by using MMTM as the backbone.}
\label{tab:nyud2-MMTM-ablation}
\center
{
\setlength{\tabcolsep}{1.9mm}
\begin{tabular}{ccc|ccccc}
\toprule
\multicolumn{1}{c}{\text{Sampling}}  & \multicolumn{1}{c}{\text{QAW}}  & \multicolumn{1}{c}{\text{$L_{reg}$}}  &
\text{$\mathbf{\epsilon=0.0}$}& \text{\begin{tabular}[c]{@{}c@{}}$\mathbf{\epsilon=10.0}$\\ \end{tabular}}& \text{\begin{tabular}[c]{@{}c@{}}$\mathbf{\epsilon=20.0}$\\ \end{tabular}}& \text{\begin{tabular}[c]{@{}c@{}}$\mathbf{\epsilon=30.0}$\\ \end{tabular}}
\\ \midrule
  
 \xmark   &\xmark         &\xmark                                          &${70.95\pm0.82}$  
       &${49.69\pm1.06}$   
       &${45.87\pm1.36}$
       &${43.88\pm1.40}$ \\
                                                                             \cmark      &\xmark  &\xmark             
                                                         &${70.80\pm0.97}$  
       &${59.79\pm1.13}$   
       &${54.74\pm1.40}$
       &${50.92\pm1.26}$                                    \\  \xmark      &\cmark  &\xmark             
                                                         &${71.86\pm0.83}$   
                                                         &${55.20\pm0.91}$   
                                                         &${49.54\pm1.26}$ 
                                                         &${47.25\pm0.72}$   \\
                                                                             \xmark      &\xmark  &\cmark             
                                                         &${72.02\pm0.67}$  
       &${54.28\pm0.50}$   
       &${47.25\pm0.98}$
       &${44.04\pm1.47}$     \\  \cmark      &\xmark  &\cmark             
                                                         &${70.49\pm0.72}$   
                                                         &${57.49\pm0.38}$   
                                                         &${51.68\pm0.16}$ 
                                                         &${50.15\pm1.59}$     \\  \cmark      &\cmark  &\xmark             
                                                         &${71.25\pm1.34}$   
                                                         &${59.33\pm0.34}$   
                                                         &${52.91\pm1.12}$ 
                                                         &${51.38\pm1.08}$    \\  \xmark      &\cmark  &\cmark             
                                                         &$\pmb{72.17\pm0.44}$   
                                                         &${54.28\pm0.57}$   
                                                         &${47.71\pm0.98}$ 
                                                         &${45.26\pm0.62}$                         \\\midrule \cmark      &\cmark  & \cmark            
                                                         &${71.56\pm1.22}$   
                                                         &${\pmb{61.47\pm0.58}}$  
                                                         &${\pmb{55.81\pm0.77}}$
                                                         &${\pmb{54.43\pm1.08}}$                                   \\ \bottomrule
\end{tabular}}
% \end{spacing}
\end{center}
\vspace{-0.4cm}
\end{table}
