# Supplementary material for: Provable Dynamic Fusion for Low-Quality Multimodal Data
Source: arXiv:2306.02050 source file (2023-06-06)
Supplement: Supplementary file 8 [file tab-classification-M3.tex]

\begin{table*}[!htbp]\small
\vspace{0.0cm}
% \vskip 0.35in
\begin{center}
% \begin{spacing}{1.05}   
\caption{Comparison with other multimodal fusion methods when $M\geq3$ in a noise regime.}
\label{tab:M3}
\center

{

\begin{tabular}{c|ccc|ccc}
\toprule \multicolumn{1}{c}{} &
\multicolumn{3}{c}{\text{ROSMAP}} & \multicolumn{3}{c}{\text{BRCA}}
\\

\toprule
\text{Method}    &
\text{ACC}& \text{\begin{tabular}[c]
{@{}c@{}}F1\\ \end{tabular}}& \text{\begin{tabular}[c]{@{}c@{}}AUC\\ \end{tabular}}& \text{\begin{tabular}[c]{@{}c@{}}ACC\\ \end{tabular}}& \text{\begin{tabular}[c]{@{}c@{}}WeightedF1\\ \end{tabular}} &\text{\begin{tabular}[c]{@{}c@{}}MacroF1\\ \end{tabular}}
\\ \toprule   \multirow{1}{*}{\text{Late fusion}}                                                         &${73.59\pm0.77}$  &${73.88\pm1.36}$  &${78.42\pm1.42}$  &${69.08\pm1.00}$   &${67.90\pm0.60}$  &${61.21\pm1.97}$                                      \\ 
       \multirow{1}{*}{\text{Concat}}                                                          &${65.72\pm2.48}$  &${66.48\pm2.07}$  &${73.60\pm0.60}$  &${67.68\pm3.24}$   &${67.22\pm3.15}$  &${61.02\pm3.56}$                                                                                                                                           \\
       \multirow{1}{*}{\text{QMF (LF)}}                                                          &  \textcolor{blue}{${77.67\pm1.18}$} &\textcolor{blue}{${78.52\pm1.52}$}  &\textcolor{blue}{${86.25\pm0.15}$}  &\textcolor{blue}{${72.88\pm0.90}$}   &\textcolor{blue}{${70.82\pm0.86}$}         &\textcolor{blue}{${65.52\pm0.42}$}                                              \\ \bottomrule
\end{tabular}}
% \end{spacing}
\end{center}
\vspace{0.0mm}
\end{table*}
